# Supplementary material for: In&Out : Diverse Image Outpainting via GAN Inversion
Source: arXiv:2104.00675 source file (2021-04-01)
Supplement: Supplementary file 1 [file 6-supp_gau_ablation.tex]

\begin{figure*}[h!]
    \centering
    \includegraphics[width=.6\linewidth]{img_sup/supp-no_prior_v1.pdf}
    \caption{
    \textbf{Qualitative ablation on using $\mathcal{L}_{\mathrm{prior}}$.} We show that, if without $\mathcal{L}_{\mathrm{prior}}$, the inversion has the risk in overfitting to the reconstruction loss with latents codes extremely far away from the training distribution. 
    The outpainted area (right part of the image) may result in direct replication of the input image.
    %, as the latent code itself carries all the structural information without utilizing the generator feature in a valid way (\ie with values in the training distribution).
    %
    In contrast, by adding the $\mathcal{L}_{\mathrm{prior}}$,
    % the additional loss regularizes the final latent codes to be located in the training distribution (\ie within a Gaussian distribution). We show that this results in a significantly better visual quality and semantically reasonable outpainting results without replicating the input image.
    we show that the outpainting results produce significantly better visual quality and semantically reasonable outpainting results without replicating the input image.
    }
    \vspace \figmargin
    \label{fig:gaussian_qual}
\end{figure*}
