# Supplementary material for: In&Out : Diverse Image Outpainting via GAN Inversion
Source: arXiv:2104.00675 source file (2021-04-01)
Supplement: Supplementary file 2 [file 6-supp_more_single.tex]

\begin{figure*}[t!]
    \centering
    \includegraphics[width=\linewidth]{example-image-a}
    \caption{
    \textbf{More inversion results.} 
    }
    \vspace \figmargin
    \label{fig:more_single}
\end{figure*}
